# Supplementary material for: Data Level Lottery Ticket Hypothesis for Vision Transformers
Source: arXiv:2211.01484 source file (2023-05-29)
Supplement: Supplementary file 1 [file 6_appendix.tex]

\section{Appendix}

\subsection{Comparisons with Existing Works}
To demonstrate the effectiveness of winning tickets, we compare our methods with the existing methods in image classification tasks, including token pruning methods and weight pruning methods. In Table~\ref{table-compare-with-other-works-at-same-gmacs}, we compare our method to several compression works with similar computation efforts on DeiT-Small~\cite{pmlr-v139-touvron21a-deit}. Our work shows the existence of the model that can achieve the best accuracy compared to other ViT compression works. For those works that train ViTs from scratch, our work shows that the LT model trained with proposed winning tickets has clear advantage in accuracy compared to the works MIA-Former~\cite{yu2022mia} and HVT~\cite{pan2021scalable}. Besides, the LT model can achieve better accuracy than the work EViT~\cite{liang2022evit} with smaller GMACs, and comparable accuracy with only half training epochs when compared to the work UVC~\cite{yu2022unified}. Furthermore, we implement the same warmup strategy as EViT in our method. The warmup strategy allows the sparsity to gradually increase from 0 to the target value with a cosine schedule during the training process, which helps our method achieve better accuracy.

\subsection{Conventional Winning Tickets in Swin Transformers}
Besides implementing experiments on normal ViTs, we also try to identify the conventional winning tickets in Swin Transformers~\cite{liu2021Swin} with the same settings as conventional LTH~\cite{frankle2018lottery}. We implement the Swin-Tiny~\cite{liu2021Swin} in the experiments and obtain the sparse mask by pruning the pretrained model weights in layers of multi-head self-attention (MSA) and MLP blocks, which is similar to the experiments conducted on DeiT-Small described in Table~\ref{weight-lth-1}. Following the conventional LTH, we train the models from scratch with the proper weight initialization (LTH) or random weight initialization (RR) and apply the same sparse mask. Also, we replace the sparse mask got from the pretrained model with a random mask (RM) to evaluate the network performance of different masks. The results are shown in Table~\ref{swin-weight-lth}. According to the results, there is no difference in accuracy between the model trained from different initializations. This indicates that there is no such unique subnetwork on weights that can be identified as a winning ticket according to the conventional LTH.

\begin{table}[t!]
\centering
\resizebox{.99\columnwidth}{!}{
\begin{tabular}{ c | c | c  c  c }
\toprule
\makecell{Weights \\ Pruned}  & \makecell{Weight \\ Sparsity} & \makecell{LTH \\ Acc. (\%)} & \makecell{RR \\ Acc. (\%)} & \makecell{Acc. \\ Diff. (\%)} \\ \midrule
None & 0\% & 81.2 & 81.2 & 0  \\ \midrule
MSA \& MLP  & 42\% & 78.9  & 78.8 & 0.1 \\ 
MSA \& MLP  & 67\% & 74.2  & 74.8 & -0.6  \\ 
\bottomrule
\end{tabular}
}
\caption{Results of experiments following conventional LTH settings on Swin-Tiny~\protect\cite{liu2021Swin}. MSA indicates the multi-head self-attention layers and MLP indicates the MLP blocks in the transformer encoder. LTH Acc. denotes the accuracy of the winning tickets (i.e., trained from the appropriate initialization); RR Acc. denotes the accuracy of the model trained from another random reinitialization; and Acc. Diff. denotes the accuracy difference between LTH Acc. and RR Acc.}
\label{swin-weight-lth}
\end{table}

\subsection{Visualization of Identified Winning Tickets in ViTs}
We visualize the identified winning tickets on the input images of ViTs in Figure~\ref{figure-visualizations} (a). Moreover, we compare the sparsified input image and the progressively sparsified results at three different stages. We implement the DynamicViT~\cite{rao2021dynamicvit} and EViT~\cite{liang2022evit} with similar computation efforts as the winning tickets for comparison.
The visualization of the DynamicViT is shown in Figure~\ref{figure-visualizations} (b) and
the EViT is shown in Figure~\ref{figure-visualizations} (c).
The figure shows that the remaining image patches of DynamicViT and EViT in the final stage are less than the winning tickets, and some attentive image patches are removed in the deep stage, which causes an accuracy drop compared to the winning tickets.

\begin{table*}[t!]
\centering
\resizebox{2.01\columnwidth}{!}{
\begin{tabular}{ c |c c c| c c c}
\toprule
Model & MACs (G) & Epochs & \makecell{Patch \\ Sparsity} & \makecell{Token \\ Sparsity} & \makecell{Weight \\ Sparsity} & Acc. (\%)  \\ \midrule
DeiT-S & 4.6  & 300 & - & - & - & 79.9 \\ \midrule
DynamicViT-DeiT-S ~\cite{rao2021dynamicvit} & 2.2 & 30 & $\times$ & \checkmark & $\times$ & 77.5 \\ 
WDPruning-DeiT-S ~\cite{fangwideanddeep} & 3.1 & 100 & $\times$ & $\times$  & \checkmark & 78.6 \\ 
WDPruning-DeiT-S ~\cite{fangwideanddeep} & 2.6 & 100 & $\times$ & $\times$  & \checkmark & 78.4 \\ 
ViT-Slim$_{PS}$-DeiT-S ~\cite{chavan2022vision} & 2.3 & 350 & $\times$ & $\times$  & \checkmark & 77.9 \\ 
EViT-DeiT-S ~\cite{liang2022evit} & 2.3 & 30 & $\times$ & \checkmark & $\times$ & 78.5 \\ \midrule
EViT-DeiT-S ~\cite{liang2022evit} & 2.3 & 300 & $\times$ & \checkmark & $\times$ & 78.5  \\ 
MIA-Former-DeiT-S ~\cite{yu2022mia} & 2.0 & - & $\times$ & \checkmark & \checkmark & 78.1  \\ 
HVT-DeiT-S ~\cite{pan2021scalable} & 2.4 & 300 & $\times$ & \checkmark & $\times$ & 78.0  \\ 
UVC-DeiT-S ~\cite{yu2022unified} & 2.3 & 600 & $\times$ & $\times$ & \checkmark & 78.8  \\ 
Ours-DeiT-S & 2.2 & 300 & \checkmark & $\times$ & $\times$ & 78.7  \\ 
Ours-DeiT-S$^{*}$ & 2.2 & 300 & \checkmark & $\times$ & $\times$ & 78.9  \\ 
\bottomrule
\end{tabular}
}
\caption{Comparisons with the existing works with comparable MACs on ImageNet.
The result with $*$ means that the same warmup strategy as EViT is used during the training progress.}
\label{table-compare-with-other-works-at-same-gmacs}
\end{table*}

\begin{figure*}[t]
    \centering
    \includegraphics[width=1.0\textwidth]{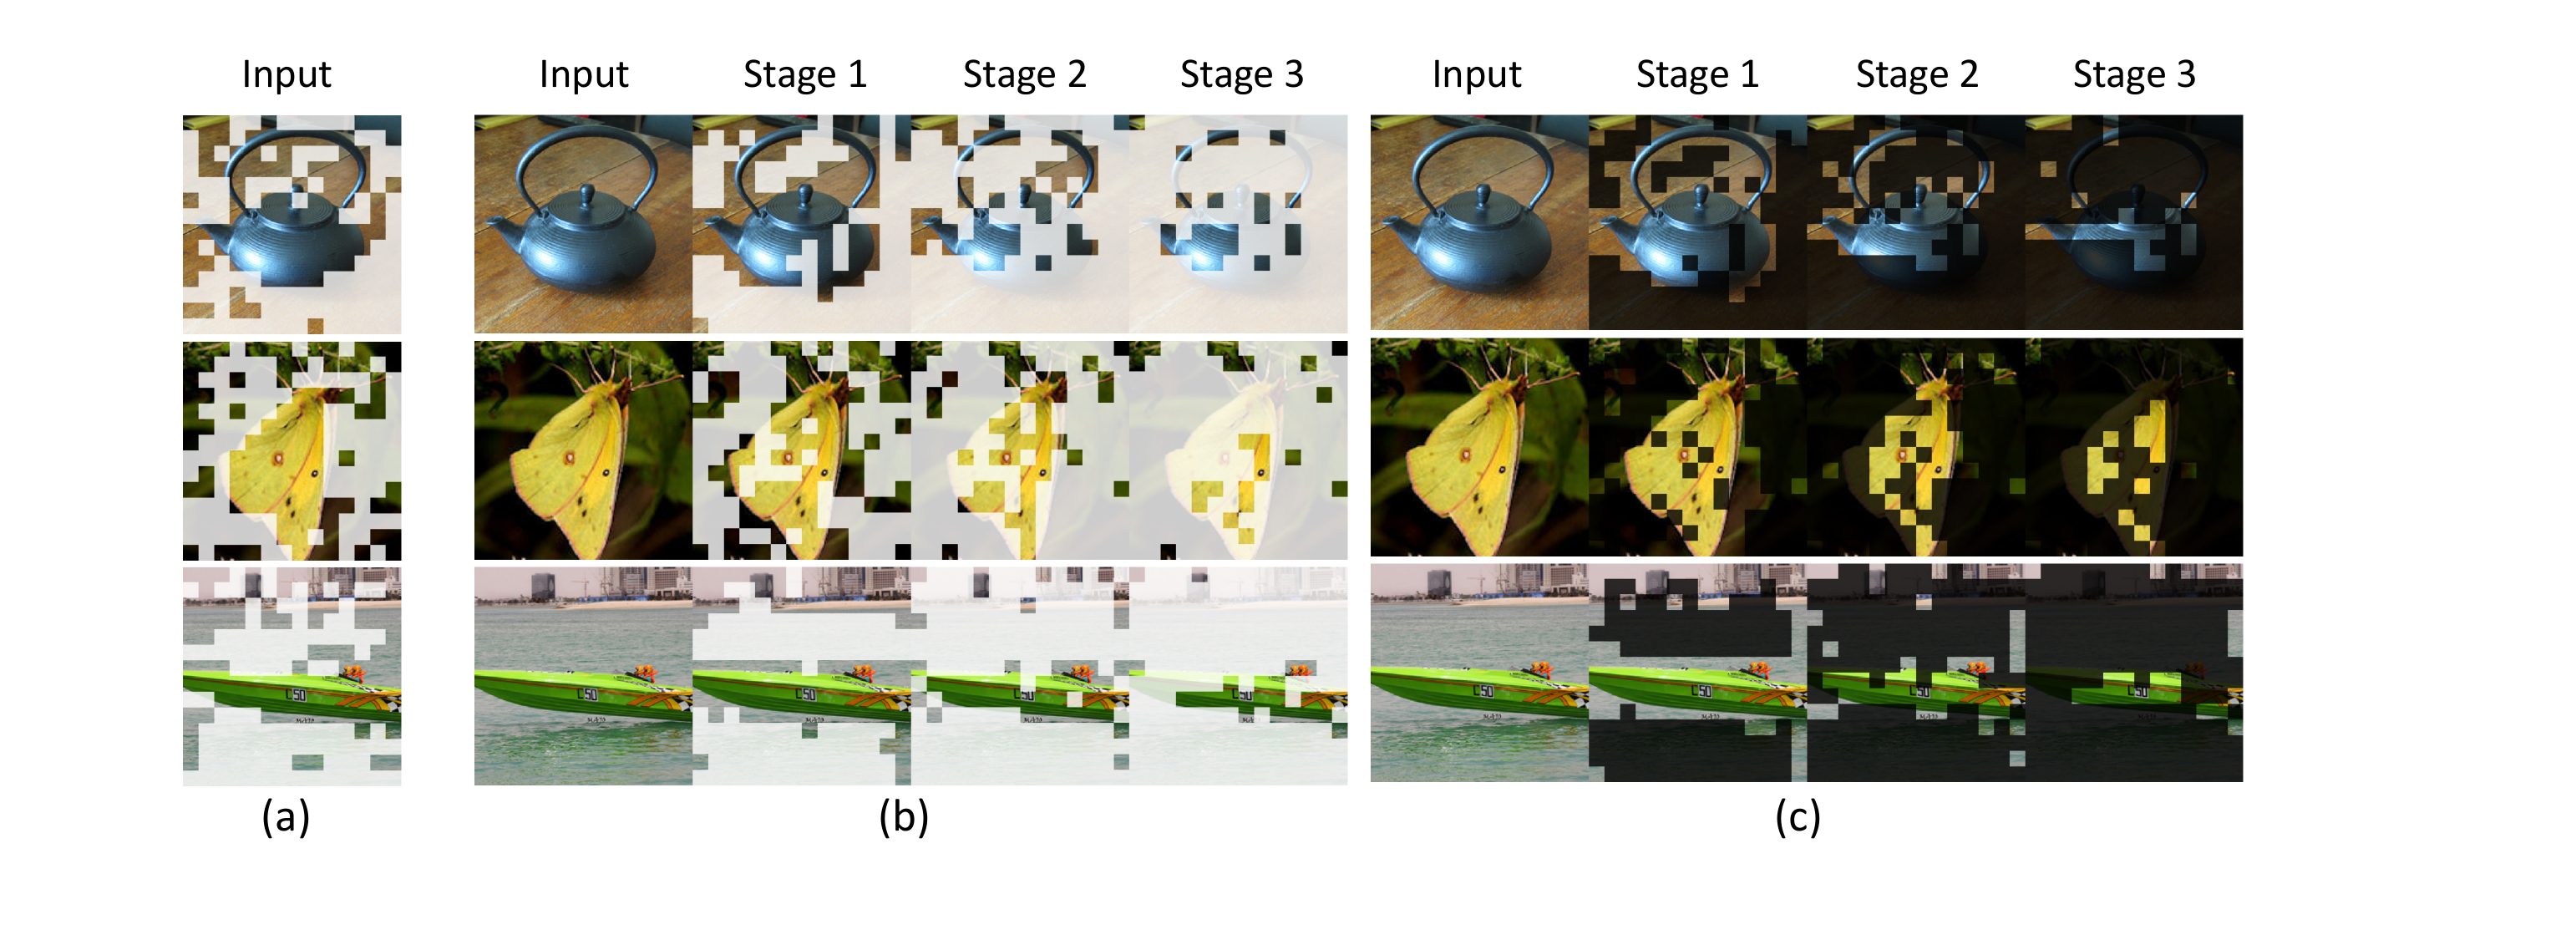}
    \caption{Visualization of the sparsified input image and progressively sparsified results. (a) Identified winning tickets, the subset of the most attentive image patches. (b) DynamicViT~\protect\cite{rao2021dynamicvit}, removing tokens at three different stages with additional token predictors. (c) EViT~\protect\cite{liang2022evit}, removing tokens at three different stages according to the importance of tokens.}
    \label{figure-visualizations}
\end{figure*}
